# Supplementary material for: Messy or Ordered? Multi-scale Mechanics DictatesShape-Morphing of Hierarchical 2D Fiber-Networks
Source: arXiv:2111.03554 ancillary file (2021-11-05)
Supplement: Supplementary file 1 [file Messy_or_Ordered_SI.pdf]

## Supplementary Information

# Messy or Ordered? Multi-scale Mechanics Dictates Shape-Morphing of Hierarchical 2D Fiber-Networks

Shiran Ziv Sharabani<sup>1,2</sup>, Nicole Edelstein-Pardo<sup>1,2</sup>, Maya Molco<sup>1,2</sup>, Michael Morami<sup>1</sup>, Netanel Bachar Schwartz<sup>1</sup>, Aya Sivan<sup>1</sup>, Eli Flaxer<sup>3</sup>, and Amit Sitt<sup>1,2,\*</sup>

<sup>1</sup>Department of Physical Chemistry, The School of Chemistry, Raymond and Beverly Sackler Faculty of Exact Sciences, Tel-Aviv University, Tel Aviv 6997801, Israel

<sup>2</sup>The Center for Nanoscience and Nanotechnology, Tel Aviv University, Tel Aviv 6997801, Israel

<sup>3</sup>AFEKA - Tel-Aviv Academic College of Engineering, 69107 Tel-Aviv, Israel

\*To whom correspondence should be addressed; E-mail: amitsitt@tauex.tau.ac.il

## Supplementary Figures

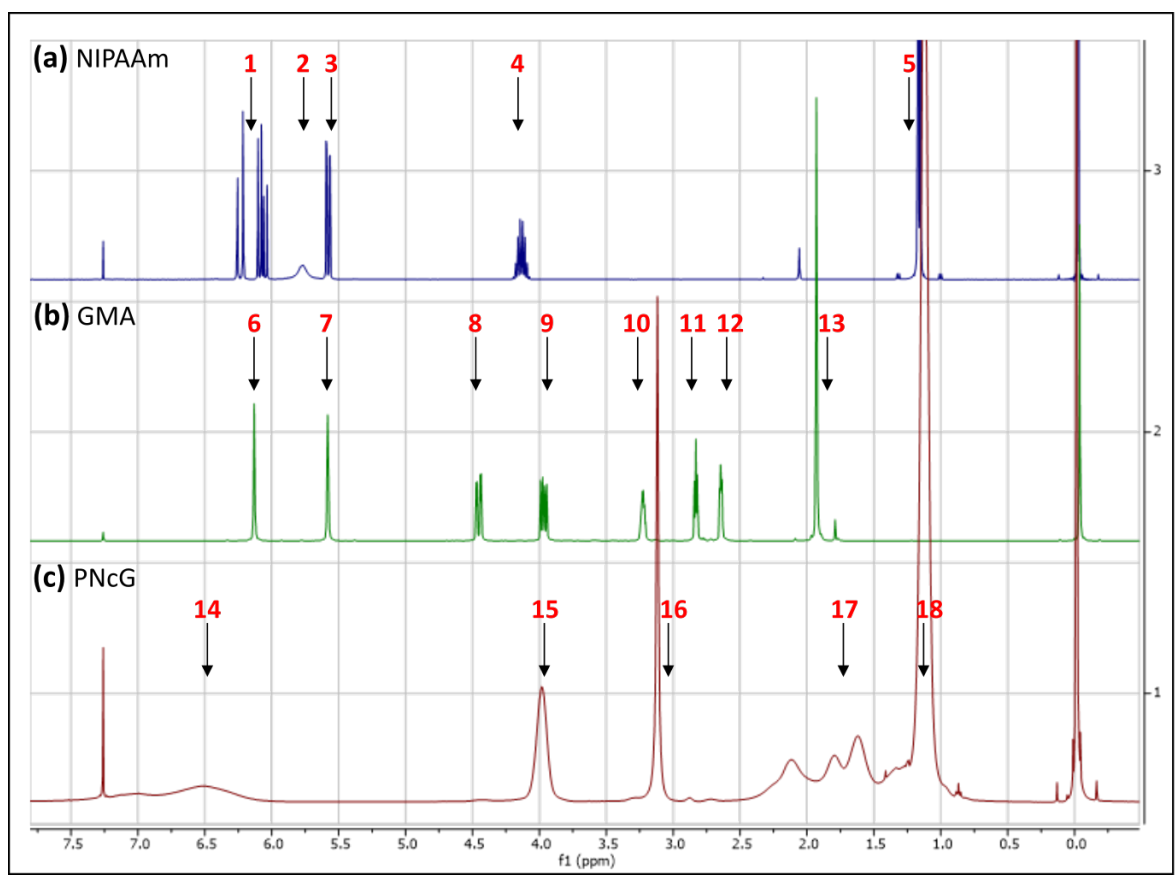

**Figure S1:**  $^1\text{H}$ -NMR spectrum of (a) the NIPAAm monomer: (400 MHz, Chloroform- $d$ )  $\delta$ : 6.27 (dd,  $J=17.0$ , 1.6Hz, 1H,  $\text{CH}_2\text{-CH-}$ ), 6.10 (dd,  $J=17.0$ , 10.2Hz, 1H,  $\text{CH}_2\text{-CH-}$ ), 5.61 (dd,  $J=10.2$ , 1.6Hz, 1H,  $\text{CH}_2\text{-CH-}$ ), 4.16 (ddt,  $J=13.1$ , 7.9, 6.6Hz, 1H,  $\text{-NH-CH-}$ ), 1.19 (dd,  $J=6.5$ , 1.2Hz, 6H,  $\text{-NH-CH(CH}_3)_2$ ). (b) The GMA monomer: (400 MHz, Chloroform- $d$ ):  $\delta$ : 6.19 – 6.14 (m, 1H,  $\text{CH}_2\text{-C(CH}_3)_2\text{O-}$ ), 5.62 (m, 1H,  $\text{CH}_2\text{-C(CH}_3)_2\text{O-}$ ), 4.49 (dd,  $J=12.3$ , 3.0 Hz, 1H,  $\text{-CO-O-CH}_2\text{-}$ ), 4.01 (dd,  $J=12.3$ , 6.2 Hz, 1H,  $\text{-CO-O-CH}_2\text{-}$ ), 3.26 (ddt,  $J=5.8$ , 4.1, 2.8Hz, 1H,  $\text{-O-CH}_2\text{-CH-}$ ), 2.87 (t,  $J=4.5$  Hz, 1H, epoxy  $\text{CH}_2$ ), 2.68 (dd,  $J=4.9$ , 2.6 Hz, 1H, epoxy  $\text{CH}_2$ ), 1.97 (t,  $J=1.4$  Hz, 3H,  $\text{CH}_2\text{-C(CH}_3)_2\text{O-}$ ). (c) PNcG: (400 MHz, Chloroform- $d$ )  $\delta$ : 6.51 (s, 1H,  $\text{-NH-}$ ), 3.98 (s, 1H,  $\text{-CO-O-CH}_2\text{-epoxy + -NH-CH-}$ ), 3.12 (s, 1H,  $\text{CH}_2\text{-C(CH}_3)_2\text{O-}$ ), 2.43 – 1.49 (m, 2H, copolymer backbone), 1.12 (s, 6H,  $\text{-NH-CH(CH}_3)_2$ ). The decrease in the intensity of peaks (1),(3),(6) and (7), which correspond to the vinyl hydrogens, confirms the polymerization of the NIPAAm and the GMA. Peak (5) that corresponds to the isopropyl in the NIPAAm monomers is maintained as peak (18). Peak (4) corresponds to the hydrogen next to the amide group in the NIPAAm, while peaks (8) – (13) correspond to the hydrogens of the glycidyl group. These peaks were most likely shifted and combined after the polymerization into peaks (15) - (16). Peak (17) corresponds to the backbone of the polymer.

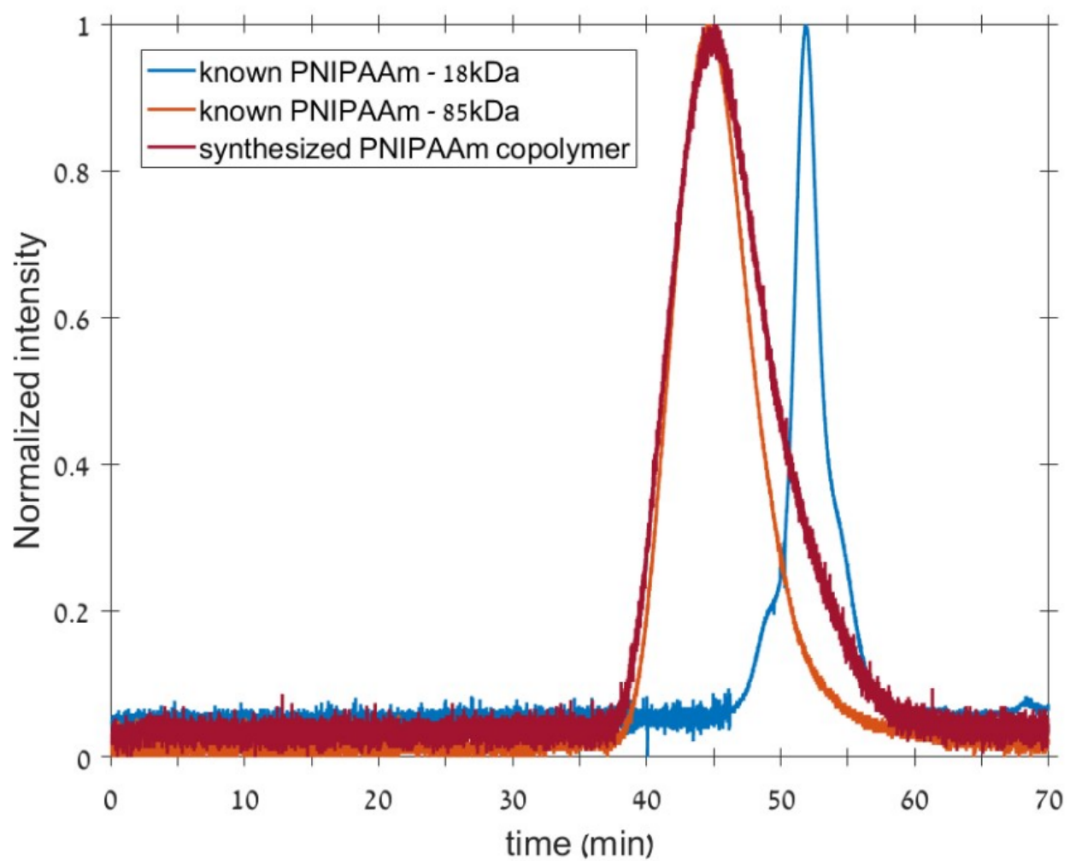

**Figure S2:** GPC results for PNIPAAm with a known molecular weights of 18 kDa (Polymer Source - product number P6699) (blue), 85 kDa (Sigma Aldrich - product number 901422) (orange), and the synthesized PNcG (red), to estimate the molecular average weight of PNcG. The synthesized copolymer had a similar retention time as the PNIPAAm with a molecular weight of 85 kDa. This result indicates that the synthesized copolymer has a molecular weight of  $\sim 85$  kDa. The peak of the copolymer is slightly broader and indicating higher dispersity.

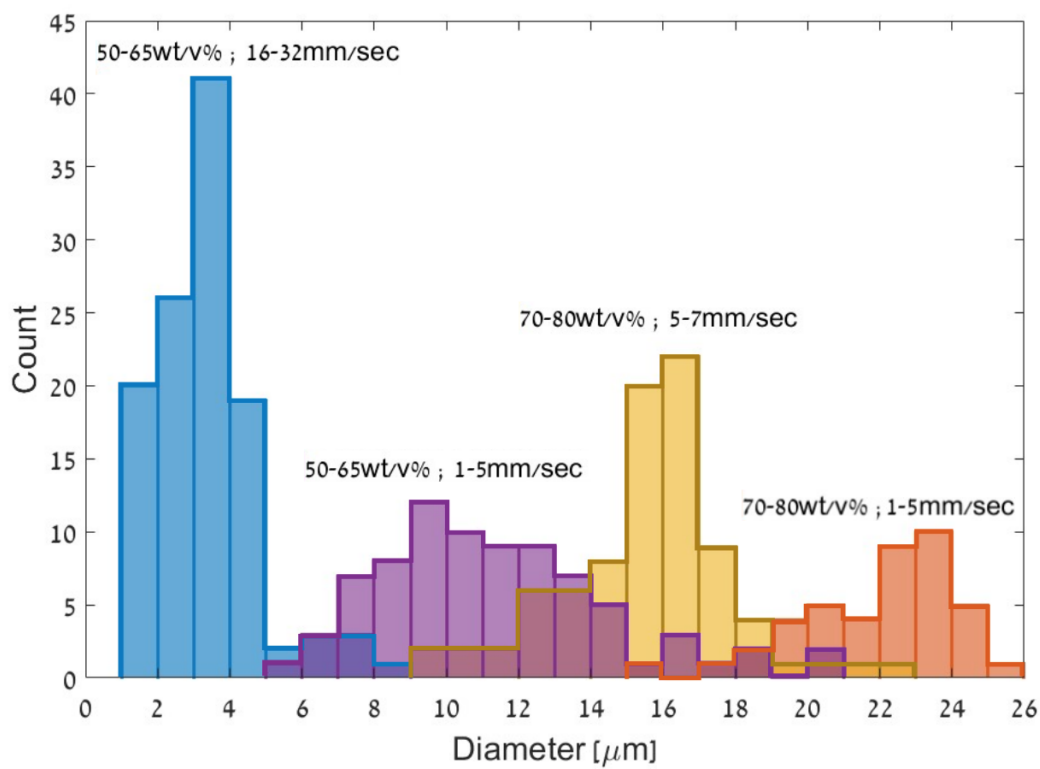

**Figure S3:** The diameter distributions of four systems of fibers extracted from SEM and optical microscope micrographs for different rotation velocities and different solution concentrations. The parameter for each sample are summarized in table S1: **(a)** Sample 1: as-spun fibers with a mean diameter of 3.4 (SD 1.4)  $\mu m$ , **(b)** sample 2: as-spun fibers with a mean diameter of 15.6 (SD 2.3)  $\mu m$ , **(c)** sample 3: as-spun fibers with a mean diameter of 11.4 (SD  $\pm 3.2$ )  $\mu m$ , and **(d)** sample 4: as-spun fibers with a mean diameter of 22.0 (SD 2.2)  $\mu m$ .

## Supplementary Tables

| # | Concentration [wt/v%] | Rotation speed [ mm/sec] | Number of measured fibers | Average fiber diameter (standard deviation) [ $\mu\text{m}$ ] |
|---|-----------------------|--------------------------|---------------------------|---------------------------------------------------------------|
| 1 | 50-65                 | 16-32                    | 80                        | 3.4 (1.4)                                                     |
| 2 | 50-65                 | 1-5                      | 115                       | 11.4 (3.2)                                                    |
| 3 | 70-80                 | 5-7                      | 85                        | 15.6 (2.3)                                                    |
| 4 | 70-80                 | 1-5                      | 42                        | 22.0 (2.2)                                                    |

**Table S1:** Summary of the diameter of the fibers that were fabricated with different parameters.

| #  | Concentration [wt/v%] | Rotation speed [mm/sec] | Crosslinker [wt/wt%] | Average fiber diameter (standard deviation) [ $\mu\text{m}$ ] | Average radius swelling ratio (standard deviation) | Average contour length swelling ratio (standard deviation) | Average order parameter (standard deviation) |
|----|-----------------------|-------------------------|----------------------|---------------------------------------------------------------|----------------------------------------------------|------------------------------------------------------------|----------------------------------------------|
| 1  | 50                    | 32                      | 6                    | 2.82 (0.53)                                                   | 3.13 (0.39)                                        | 1.43(0.14)                                                 | 0.86 (0.12)                                  |
| 2  | 50                    | 32                      | 10                   | 3.93 (0.69)                                                   | 3.18 (0.49)                                        | 1.99(0.90)                                                 | 0.80 (0.16)                                  |
| 3  | 50                    | 32                      | 6                    | 4.68 (0.64)                                                   | 1.70 (0.23)                                        | 1.83(0.15)                                                 | 0.81 (0.16)                                  |
| 4  | 55                    | 27                      | 6                    | 5.06 (0.64)                                                   | 1.89 (0.37)                                        | 1.95(0.18)                                                 | 0.78 (0.21)                                  |
| 5  | 50                    | 27                      | 6                    | 5.13 (0.68)                                                   | 2.40 (0.31)                                        | 2.18(0.15)                                                 | 0.76 (0.21)                                  |
| 6  | 55                    | 13                      | 6                    | 5.33 (0.43)                                                   | 1.86 (0.37)                                        | 1.87(0.10)                                                 | 0.80 (0.16)                                  |
| 7  | 65                    | 32                      | 6                    | 5.94 (0.26)                                                   | 3.11 (0.26)                                        | 1.43(0.15)                                                 | 0.906(0.085 )                                |
| 8  | 60                    | 32                      | 2                    | 6.06 (0.88)                                                   | 2.46 (0.37)                                        | 1.98(0.22)                                                 | 0.940(0.067 )                                |
| 9  | 55                    | 27                      | 6                    | 6.29 (0.79)                                                   | 2.16 (0.39)                                        | 2.04(0.39)                                                 | 0.80 (0.17)                                  |
| 10 | 65                    | 32                      | 6                    | 6.69 (0.37)                                                   | 2.06 (0.14)                                        | 2.04(0.15)                                                 | 0.892(0.094 )                                |
| 11 | 60                    | 32                      | 6                    | 7.1 (1.4)                                                     | 2.22 (0.34)                                        | 2.25 (0.15)                                                | 0.958 (0.046)                                |
| 12 | 70                    | 5                       | 6                    | 11.8 (1.3)                                                    | 2.09 (0.35)                                        | 1.491 (0.063)                                              | 0.9970 (0.0045)                              |
| 13 | 55                    | 32                      | 6                    | 13.0 (2.0)                                                    | 1.64 (0.40)                                        | 1.541(0.087 )                                              | 0.964 (0.019)                                |
| 14 | 50                    | 3                       | 6                    | 15.3 (3.2)                                                    | 1.99 (0.41)                                        | 1.489(0.093 )                                              | 0.983 (0.015)                                |
| 15 | 80                    | 5                       | 6                    | 22.5 (2.1)                                                    | 2.28 (0.25)                                        | 1.63 (0.16)                                                | 0.993 (0.012)                                |
| 16 | 70                    | 6                       | 6                    | 23.0 (2.3)                                                    | 2.37 (0.24)                                        | 1.70 (0.15)                                                | 0.9915 (0.0055)                              |
| 17 | 80                    | 5                       | 6                    | 26.1 (2.9)                                                    | 2.15 (0.24)                                        | 1.63 (0.10)                                                | 0.9957 (0.0049)                              |
| 18 | 80                    | 4                       | 6                    | 28.0 (1.7)                                                    | 2.18 (0.73)                                        | 1.594 (0.051)                                              | 0.9941 (0.0070)                              |
| 19 | 70                    | 5                       | 1                    | 30.2 (3.5)                                                    | 2.87 (0.25)                                        | 2.09 (0.26)                                                | 0.986 (0.010)                                |
| 20 | 55                    | 27                      | 6                    | 5.0 (1.4)                                                     | 1.58 (0.31)                                        | 2.05 (0.20)                                                | 0.984 (0.018)                                |

**Table S2:** The analyzed networks that were examined in this research, the fabrication parameters and the obtained networks parameters. The microfibers of the crosslinked copolymer exhibited different swelling ratios along and in perpendicular of the main axes of the fiber. The longitudinal swelling ratio of the fiber is defined as the ratio between the average contour length of the fiber below the LCST,  $l_{cold}$ , and above the LCST,  $l_{hot}$ ,  $q_l = l_{cold}/l_{hot}$  and the average longitudinal swelling is  $q_l = 1.79$  (SD 0.26). The transverse swelling ratio (in perpendicular to the main axis of the fiber) is defined as the ratio between the average radius of the fiber below the LCST,  $r_{cold}$ , and above the LCST,  $r_{hot}$ ,  $q_r = r_{cold}/r_{hot}$ . The average transverse swelling is  $q_r = 2.30$  (SD 0.45).

## Supplementary Notes

### 1. Network's Projected Area to Fiber Elongation Ratio

Another indicator for the transition in morphing behaviors is the relation between the swelling ratio of the network itself,  $Q_S$ , and the average squared swelling ratio of the fibers constructing the network,  $q_l^2$ .  $Q_S$ , is defined as the ratio between the total area of the network below the LCST, and above the LCST. The network projected area was defined as the tetragon obtained by connecting the four nodes that form the corners of the original Cartesian network. For the shape-preserving network,  $Q_S/q_l^2 \sim 1$ , because the elongation of the fibers almost fully translates to the extension of the network itself. However, when the fibers buckle upon swelling, the extension of the network can be significantly reduced. Fig. 3d depicts  $Q_S/q_l^2$  as function of the fiber diameter for networks with density of 5.6 fibers per millimeter above the LCST with a standard deviation of 2.3. For networks constructed of fibers with diameters above  $7 \mu m$  the ratio is  $\sim 1$ , indicating that these are shape-preserving networks. However, below these diameters, the ratio decreases as the diameter of the fibers decreases, indicating a decrease in the contribution of fiber elongation to the extension of the entire network.

### 2. Detailed description of the numerical model

The persistence length,  $p_l$ , of a stiff filament is given by:

$$p_l = \frac{E\pi r^4}{4k_B T}, \quad (1)$$

where  $k_B$  is the Boltzmann constant. Plugging in the Young modulus of PNIPAAm,  $E = 29.4 kPa$ , for a filament with a radius of  $r = 1 \mu m$  at room temperature, the calculated persistence length is  $4.8 m$ . Hence, we do not expect thermal effects to contribute considerably to the morphing behavior, and the network can be expressed as an overdamped system in a viscous medium<sup>1</sup>.

Estimation of Young modulus of the swelled fibers, Flory-Rehner equation is used<sup>2</sup>:

$$-[\ln(1 - \phi) + \phi + \chi\phi^2] = V_1 \frac{\rho}{M_c} \left[ \phi^{\frac{1}{3}} - \frac{\phi}{2} \right], \quad (2)$$

where  $\phi$  is the fraction of the polymer in the solution  $V_1$  is the molar volume of the solvent (water),  $\rho$  is the PNIPAAm density, and  $M_c$  is the average molecular weight of the polymer segments.  $M_c$  can be divided by the molecular weight of one monomer to obtain  $N_{gel}$ , the number of monomers between two crosslinks.  $\chi$  is the Flory-Huggins parameter, and is empirically expressed as:

$$\chi = \chi_1(T) + \chi_2(\phi) + O(\phi^2). \quad (3)$$

$\chi_1$  and  $\chi_2$  are given by:

$$\chi_1 = \frac{1}{2} - A \left( 1 - \frac{T_c}{T} \right); \chi_2 = C\phi, \quad (4)$$

where  $A$  holds the entropic contributions that are not related to the mixing and is determined empirically,  $C$  is an empirical constant that is independent of the temperature, and  $T_c$  it the LCST of PNIPAAm. The Flory-Renher model also allows extracting the shear and bulk moduli ( $\mu$  and  $K$  respectively):

$$\mu = \left( \frac{\phi k_B T}{2N_{gel}\alpha^3} \right) \left( \frac{\phi}{\phi_0} \right)^{1/3}, \quad (5)$$

$$K = \frac{k_B T}{\alpha^3} \left[ \frac{\phi^2}{1-\phi} - 2\chi_1\phi^2 - 3\chi_2\phi^3 + \frac{\phi_0}{N_{gel}} \left( \frac{\phi}{2\phi_0} - \frac{1}{3} \left( \frac{\phi}{\phi_0} \right)^{1/3} \right) \right], \quad (6)$$

where  $\alpha$  is the monomer length.  $\phi_0$  is the polymer volume fraction at the reference state (or at the collapsed state above the LCST), and is usually set to 1. The Young modulus can be calculated from both of the moduli:

$$E = \frac{9K\mu}{3K + \mu}. \quad (7)$$

Here, we used to following parameters:  $\phi = \frac{1}{Q}$ , where  $Q$  is the swelling ratio of the fibers in 3D. Based on our result,  $q_r = 2.5$  and  $q_l = 1.75$ . Due to the cylindrical geometry of the fiber, the swelling ratio of the total volume is 10.94, and therefore  $\phi = 0.0914$ . The parameters  $A$  and  $C$  where taken as  $-1$  and  $0.32$  respectively, based on previous studies on PNIPAAm<sup>3</sup>. For those parameters, the calculated Young modulus is  $29.4 \text{ kPa}$  for the fiber at the swollen state.

### Movie S1

Shape-morphing video of a shape-preserving network in aqueous environment (sample 16, Table S2). The video includes both the cooling process (played at 8x speed) from  $60^\circ\text{C}$  to  $25^\circ\text{C}$  and the heating process (played at 2x speed) from  $25^\circ\text{C}$  to  $60^\circ\text{C}$  of the network.

### Movie S2

Shape-morphing video of a buckling-governed network in aqueous environment (sample 2, Table S2). The video includes both the cooling process (played at 4x speed) from  $60^\circ\text{C}$  to  $25^\circ\text{C}$  and the heating process (played at 2x speed) from  $25^\circ\text{C}$  to  $60^\circ\text{C}$  of the network.

## References

1. Kim, T., Hwang, W., Lee, H. & Kamm, R. D. Computational analysis of viscoelastic properties of crosslinked actin networks. *PLoS Computational Biology* **5**, e1000439 (2009).
2. Flory, P. J. *Principles of polymer chemistry chap. 13* (1953).
3. Lopez, C. G. & Richtering, W. Does Flory-Rehner theory quantitatively describe the swelling of thermoresponsive microgels? *Soft Matter* **13**, 8271–8280 (2017).
